# Supplementary material for: Geometry-aware neural solver for fast Bayesian calibration of brain tumor models
Source: arXiv:2009.04240 source file (2021-04-14)
Supplement: Supplementary file 1 [file suppl.tex]

%\section{}


% \begin{figure*}[h]
% \begin{subfigure}{0.33\textwidth}
% \includegraphics[width=\linewidth]{dice20_geom_3_extracsf_1tissue.png}
% \caption{DICE $>$ 0.2}
% \end{subfigure}%
% \begin{subfigure}{0.33\textwidth}
% \includegraphics[width=\linewidth]{dice40_geom_3_extracsf_1tissue.png}
% \caption{DICE $>$ 0.4}
% \end{subfigure}%
% \begin{subfigure}{0.33\textwidth}
% \includegraphics[width=\linewidth]{dice80_geom_3_extracsf_1tissue.png}
% \caption{DICE $>$ 0.8}
% \end{subfigure}%

% \caption{Ablation analysis I. Instead of inputting 3 volumes of different tissue types (WM, GM, CSF) only a single volume of CSF tissue serves as an input to the network. The figure shows the histograms of the DICE score computed on the whole validation set for the tumor volumes $\mathbf{u}_{\mathit{pred}}$ and $\mathbf{u}_{\mathit{sim}}$ thresholded at 0.2, 0.4, and 0.8 values of tumor cell concentration. The means of the distributions are: a) 0.798, b) 0.799, c) 0.801. } 
% \label{fig12}
% \end{figure*}

% \begin{figure*}[h]
% \begin{subfigure}{0.33\textwidth}
% \includegraphics[width=\linewidth]{dice20_1loss_orig.png}
% \caption{DICE $>$ 0.2}
% \end{subfigure}%
% \begin{subfigure}{0.33\textwidth}
% \includegraphics[width=\linewidth]{dice40_1loss_orig.png}
% \caption{DICE $>$ 0.4}
% \end{subfigure}%
% \begin{subfigure}{0.33\textwidth}
% \includegraphics[width=\linewidth]{dice80_1loss_orig.png}
% \caption{DICE $>$ 0.8}
% \end{subfigure}%

% \caption{Ablation analysis II. Instead of splitting the $L_\mathbf{total}$ into two terms as in Eq. 3, a standard L1 loss is used for computing the error in the whole volume. The figure shows the histograms of the DICE score computed on the whole validation set for the tumor volumes $\mathbf{u}_{\mathit{pred}}$ and $\mathbf{u}_{\mathit{sim}}$ thresholded at 0.2, 0.4, and 0.8 values of tumor cell concentration.} 
% \label{fig13}
% \end{figure*}


%##############################################################################

% \begin{figure*}[h]
% \begin{subfigure}{0.2\textwidth}
% \includegraphics[width=\linewidth]{mre_0.05-0.2_small.png}
% \end{subfigure}%
% \begin{subfigure}{0.2\textwidth}
% \includegraphics[width=\linewidth]{mre_0.2-0.4_small.png}
% \end{subfigure}%
% \begin{subfigure}{0.2\textwidth}
% \includegraphics[width=\linewidth]{mre_0.4-0.6_small.png}
% \end{subfigure}%
% \begin{subfigure}{0.2\textwidth}
% \includegraphics[width=\linewidth]{mre_0.6-0.8_small.png}
% \end{subfigure}%
% \begin{subfigure}{0.2\textwidth}
% \includegraphics[width=\linewidth]{mre_0.8-1.0_small.png}
% \end{subfigure}%
% \subcaption{small}


% \begin{subfigure}{0.2\textwidth}
% \includegraphics[width=\linewidth]{mre_0.05-0.2_middle.png}
% \end{subfigure}%
% \begin{subfigure}{0.2\textwidth}
% \includegraphics[width=\linewidth]{mre_0.2-0.4_middle.png}
% \end{subfigure}%
% \begin{subfigure}{0.2\textwidth}
% \includegraphics[width=\linewidth]{mre_0.4-0.6_middle.png}
% \end{subfigure}%
% \begin{subfigure}{0.2\textwidth}
% \includegraphics[width=\linewidth]{mre_0.6-0.8_middle.png}
% \end{subfigure}%
% \begin{subfigure}{0.2\textwidth}
% \includegraphics[width=\linewidth]{mre_0.8-1.0_middle.png}
% \end{subfigure}%
% \subcaption{medium}


% \begin{subfigure}{0.2\textwidth}
% \includegraphics[width=\linewidth]{mre_0.05-0.2_large.png}
% \end{subfigure}%
% \begin{subfigure}{0.2\textwidth}
% \includegraphics[width=\linewidth]{mre_0.2-0.4_large.png}
% \end{subfigure}%
% \begin{subfigure}{0.2\textwidth}
% \includegraphics[width=\linewidth]{mre_0.4-0.6_large.png}
% \end{subfigure}%
% \begin{subfigure}{0.2\textwidth}
% \includegraphics[width=\linewidth]{mre_0.6-0.8_large.png}
% \end{subfigure}%
% \begin{subfigure}{0.2\textwidth}
% \includegraphics[width=\linewidth]{mre_0.8-1.0_small.png}
% \end{subfigure}%
% \subcaption{large}

% \caption{Histograms of the mean relative error per sample between the predicted by the surrogate and simulated tumor volumes computed on the whole validation set. To calculate the error both tumors were divided into 5 various tumor concentration regions: 0-0.2, 0.2-0.4, 0.4-0.6, 0.6-0.8, 0.8-1.0. The rows represent a) small (less than 20$\%$ of the 64x64x64 volume), b) medium (between 20$\%$ and 60$\%$), and c) large (greater than 60$\%$) tumors. } 
% \label{fig10}
% \end{figure*}

% \begin{figure}[h]
% \centering
% {\includegraphics[width=\columnwidth]{last_geom_param_plot_1.pdf}}{Simulation b}
% \\

% {\includegraphics[width=\columnwidth]{last_geom_param_plot_2.pdf}}{\ \ \ \ \ \ \ \ \ Simulation a}
% \caption{Predicted tumor volumes and corresponding simulated ground truths (in green). For  all  columns  the  network  input parameters ${D,\rho}$ and the brain anatomy are fixed, whereas each column has a different value of $T$ from 300 to 1000 days with intervals of 100 days. The images were obtained by inferring individual 3D volumes (in a single batch) for all time values and taking a central 2D slice from each volume. The last rows framed in green correspond to the ground truth simulation.} \label{fig8}
%\end{figure}

% \begin{figure}[h]
% \includegraphics[width=\columnwidth]{pairwise.png}
% % \includegraphics[width=0.5\textwidth]{tumor_crossed_gt.pdf}
% \caption{Comparison between the Bayesian personalization using numerical and neural solvers. Along the diagonal marginal distributions for neural (solid blue line) and numerical (orange dotted line) are shown. Above the diagonal - joint posterior distributions for a pair of corresponding model parameters as red contours and green heat-map for neural and numerical solver, respectively.} \label{fig3}
% \end{figure}
